# Supplementary material for: Efficient Training of Visual Transformers with Small Datasets
Source: arXiv:2106.03746 source file (2021-11-14)
Supplement: Supplementary file 1 [file code-deterministic-full.tex]

\begin{minted}[
fontsize=\fontsize{8.5}{9},
frame=single,
framesep=2.5pt,
baselinestretch=1.05,
]{python}
def position_sampling(bsz, N):
    all_positions = [[i,j]  for i in range(N) for j in range(N)]
    pts = torch.tensor(all_positions) # [N*N, 2]
    pos_1 = pts.repeat(bsz,1,1)  # [B, N*N, 2]
    rnd_idx = torch.stack([torch.randperm(N*N) for _ in range(bsz)], dim=0) # [B, N*N]
    pos_2 = torch.stack([pos_1[idx,r] for idx, r in enumerate(rnd_idx)],dim=0) # [B, N*N, 2]
    return pos_1, pos_2
\end{minted}
