# Supplementary material for: Efficient Training of Visual Transformers with Small Datasets
Source: arXiv:2106.03746 source file (2021-11-14)
Supplement: Supplementary file 2 [file code-pixelsame.tex]

\begin{minted}[
fontsize=\fontsize{8.5}{9},
frame=single,
framesep=2.5pt,
baselinestretch=1.05,
]{python}
    def forward(self, x):
        bsz, D, N, N = x.size()
        pos_1, pos2 = position_sampling(N, self.sz, bsz, x.device)
        pts_1 = collect_samples(x, pos_1, bsz).transpose(1,2).contiguous() # [bsz, sz, D]
        pts_2 = collect_samples(x, pos_2, bsz).transpose(1,2).contiguous() # [bsz, sz, D]
        
        pts_1, pts_2 = pts_1.view(-1, D), pts_2.view(-1, D) # [bsz*sz, C], [bsz*sz, D]
        rnd_idx = torch.arange(bsz).roll(1)
        pos_3 = pos_1[rnd_idx]
        pts_3 = collect_samples(x[rnd_idx], pos_3, bsz).transpose(1,2) # [bsz, sz, D]
        pts_3 = pts_3.contiguous().view(-1, D) # [bsz*sz, D]
        
        pos_pairs = torch.cat([pts_1, pts_2], dim=1) # [bsz*sz, D*2]
        neg_pairs = torch.cat([pts_1, pts_3], dim=1) # [bsz*sz, D*2]
        labels = torch.cat([torch.ones(bsz*self.sz), torch.zeros(bsz*self.sz)],dim=0)
        labels = labels.long().to(x.device)
        
        rnd_idx = torch.randperm(labels.size(0))
        logits = self.layer(torch.cat([pos_pairs, neg_pairs],dim=0)[rnd_idx])
        target = labels[rnd_idx]
        return logits, target
\end{minted}
